# Supplementary material for: Infinite Mobility: Scalable High-Fidelity Synthesis of Articulated Objects via Procedural Generation
Source: arXiv:2503.13424 source file (2025-03-17)
Supplement: Supplementary file 1 [file X_suppl.tex]

\clearpage
\appendixpage
\addappheadtotoc
\setcounter{page}{1}
% \maketitlesupplementary
% \twocolumn[
% \centering
% \Large
% %\textbf{\thetitle}\\
% \vspace{0.5em}Supplementary Material \\
% \vspace{1.0em}
% ]%< twocolumn 
%\tableofcontents
\appendix
\section{All Categories We Support}
In this section, we provide the list of all categories we support in Infinite Mobility till now.
Based on frequency of interactions we observed and difficulty of implementation, we selected 22 categories of objects.
\begin{itemize}
    \item Cabinet
    \item Pan
    \item Pot
    \item TV(Display)
    \item Dishwasher
    \item Microwave
    \item Fridge
    \item Oven
    \item Bar Chair
    \item Office Chair
    \item Window
    \item Lamp
    \item Tap
    \item Toilet
    \item Hardware
    \item Door
    \item Rack
    \item Cocktail Table
    \item Dining Table
    \item Plate Rack
    \item Bottle
    \item Vase
\end{itemize}

\section{Detail of Human Evaluation}
In this section, we provide the details in the human evaluation.
When completing the evaluation, the annotators were asked to answer the following question after watching each pair of videos .
%\vspace{-1em}
\begin{figure}[!h]
    \centering
    \includegraphics[width=1\linewidth]{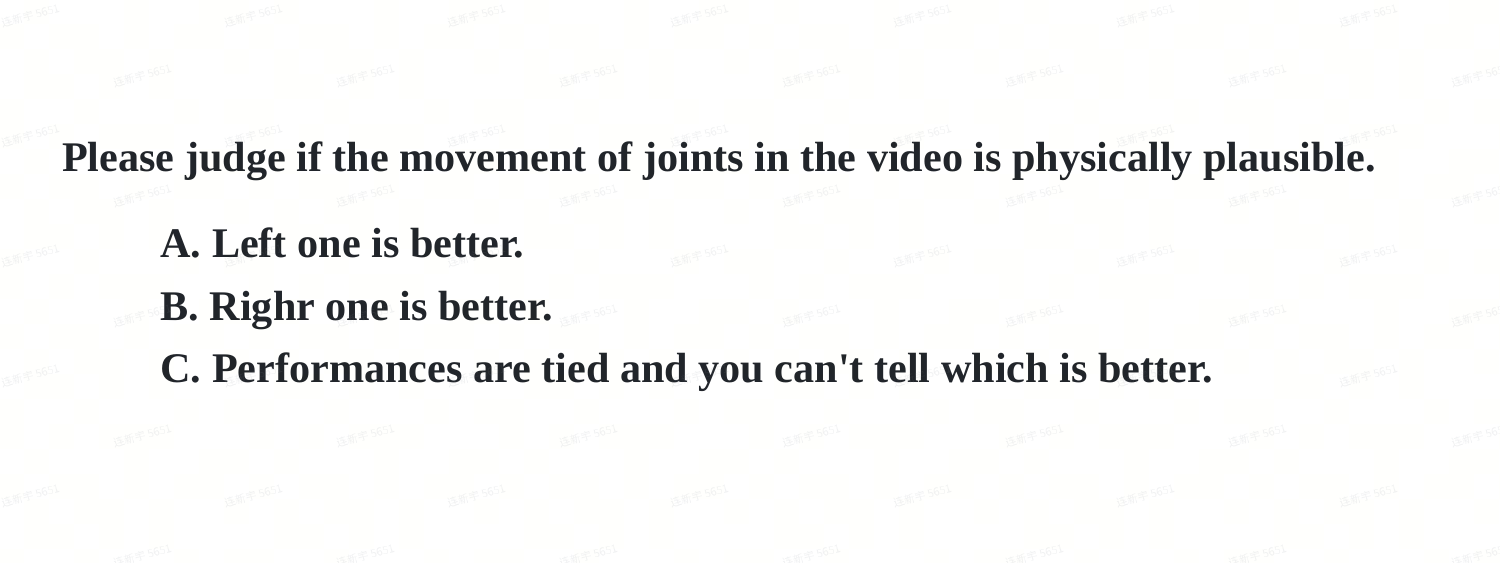}
    \vspace{-2em}
    \caption{Question used in human evaluation.}
    \label{fig:human_evaluation}
\end{figure}
For each category, we construct 50 pairs of videos for evaluation.
For PartNet-Mobility, if sample in one category is not available, we may use one sample for multiple times.
For NAP, due to that it can't be conditioned on categories, we randomly select 50 samples from all categories.
%5We conduct the evaluation in the form of questionnaires, each questionnaire contains 50 valid pairs and 10 biased pairs which are used to judge the quality of answers.
%A sample of biased pairs is shown in Figure~\ref{fig:biased_question}.
% \begin{figure}
%     \vspace{-1em}
%     \centering
%     \includegraphics[width=1\linewidth]{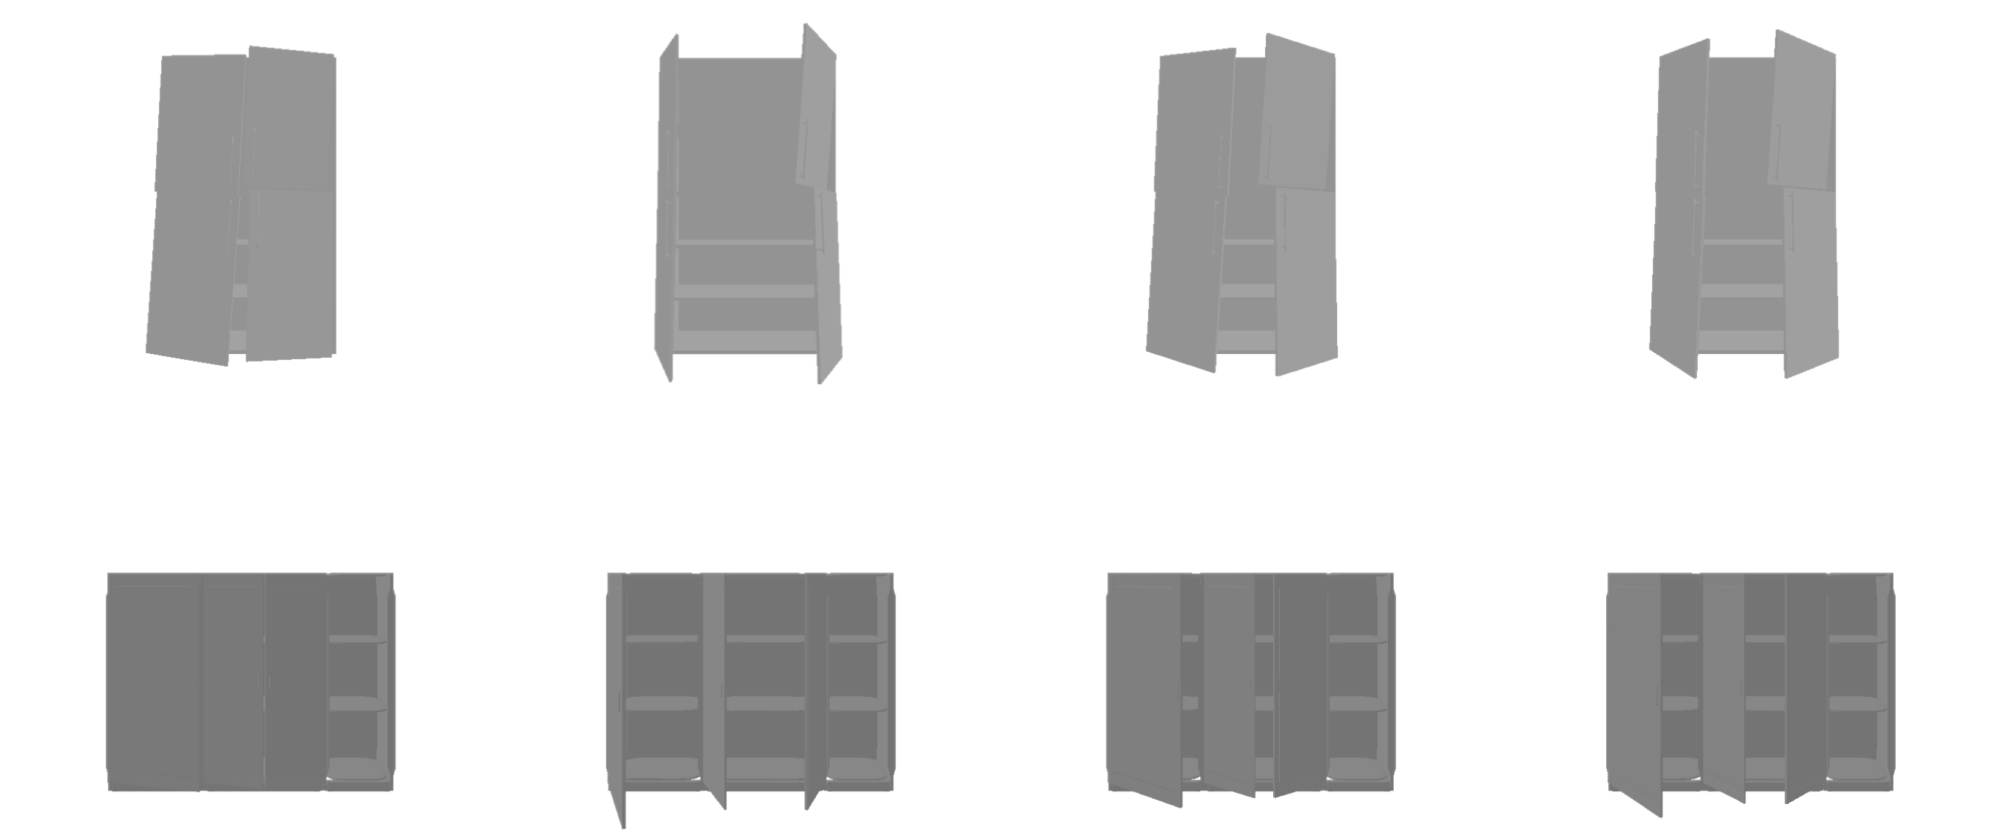}
%     \caption{Biased sample pair for human evaluation.}
%     \label{fig:biased_question}
% \end{figure}
%In evaluation comparing our results and PartNet-Mobility, we created 15 questionnairs for each category and 6 questionnairs with objects from all categories.
%In evaluation comparing our results with CAGE, we created 6 questionnairs for each category and 6 questionnairs with objects from all categories.
%In evaluation comparing our results with NAP, we created 6 questionnairs ignoring categories.
%In all answers collected, less than 5\% of the biased pairs are wrongly judged.

\section{Detail of GPT4v Evaluation}
In this section, we provide the details of the evaluation of mesh quality using GPT4v.
We render normal maps and RGB images for each articulated object and construct paired samples for comparison.
One sample pair is shown in Figure~\ref{fig: gpt4v_samples}.
\begin{figure}
    \centering
    \includegraphics[width=1\linewidth]{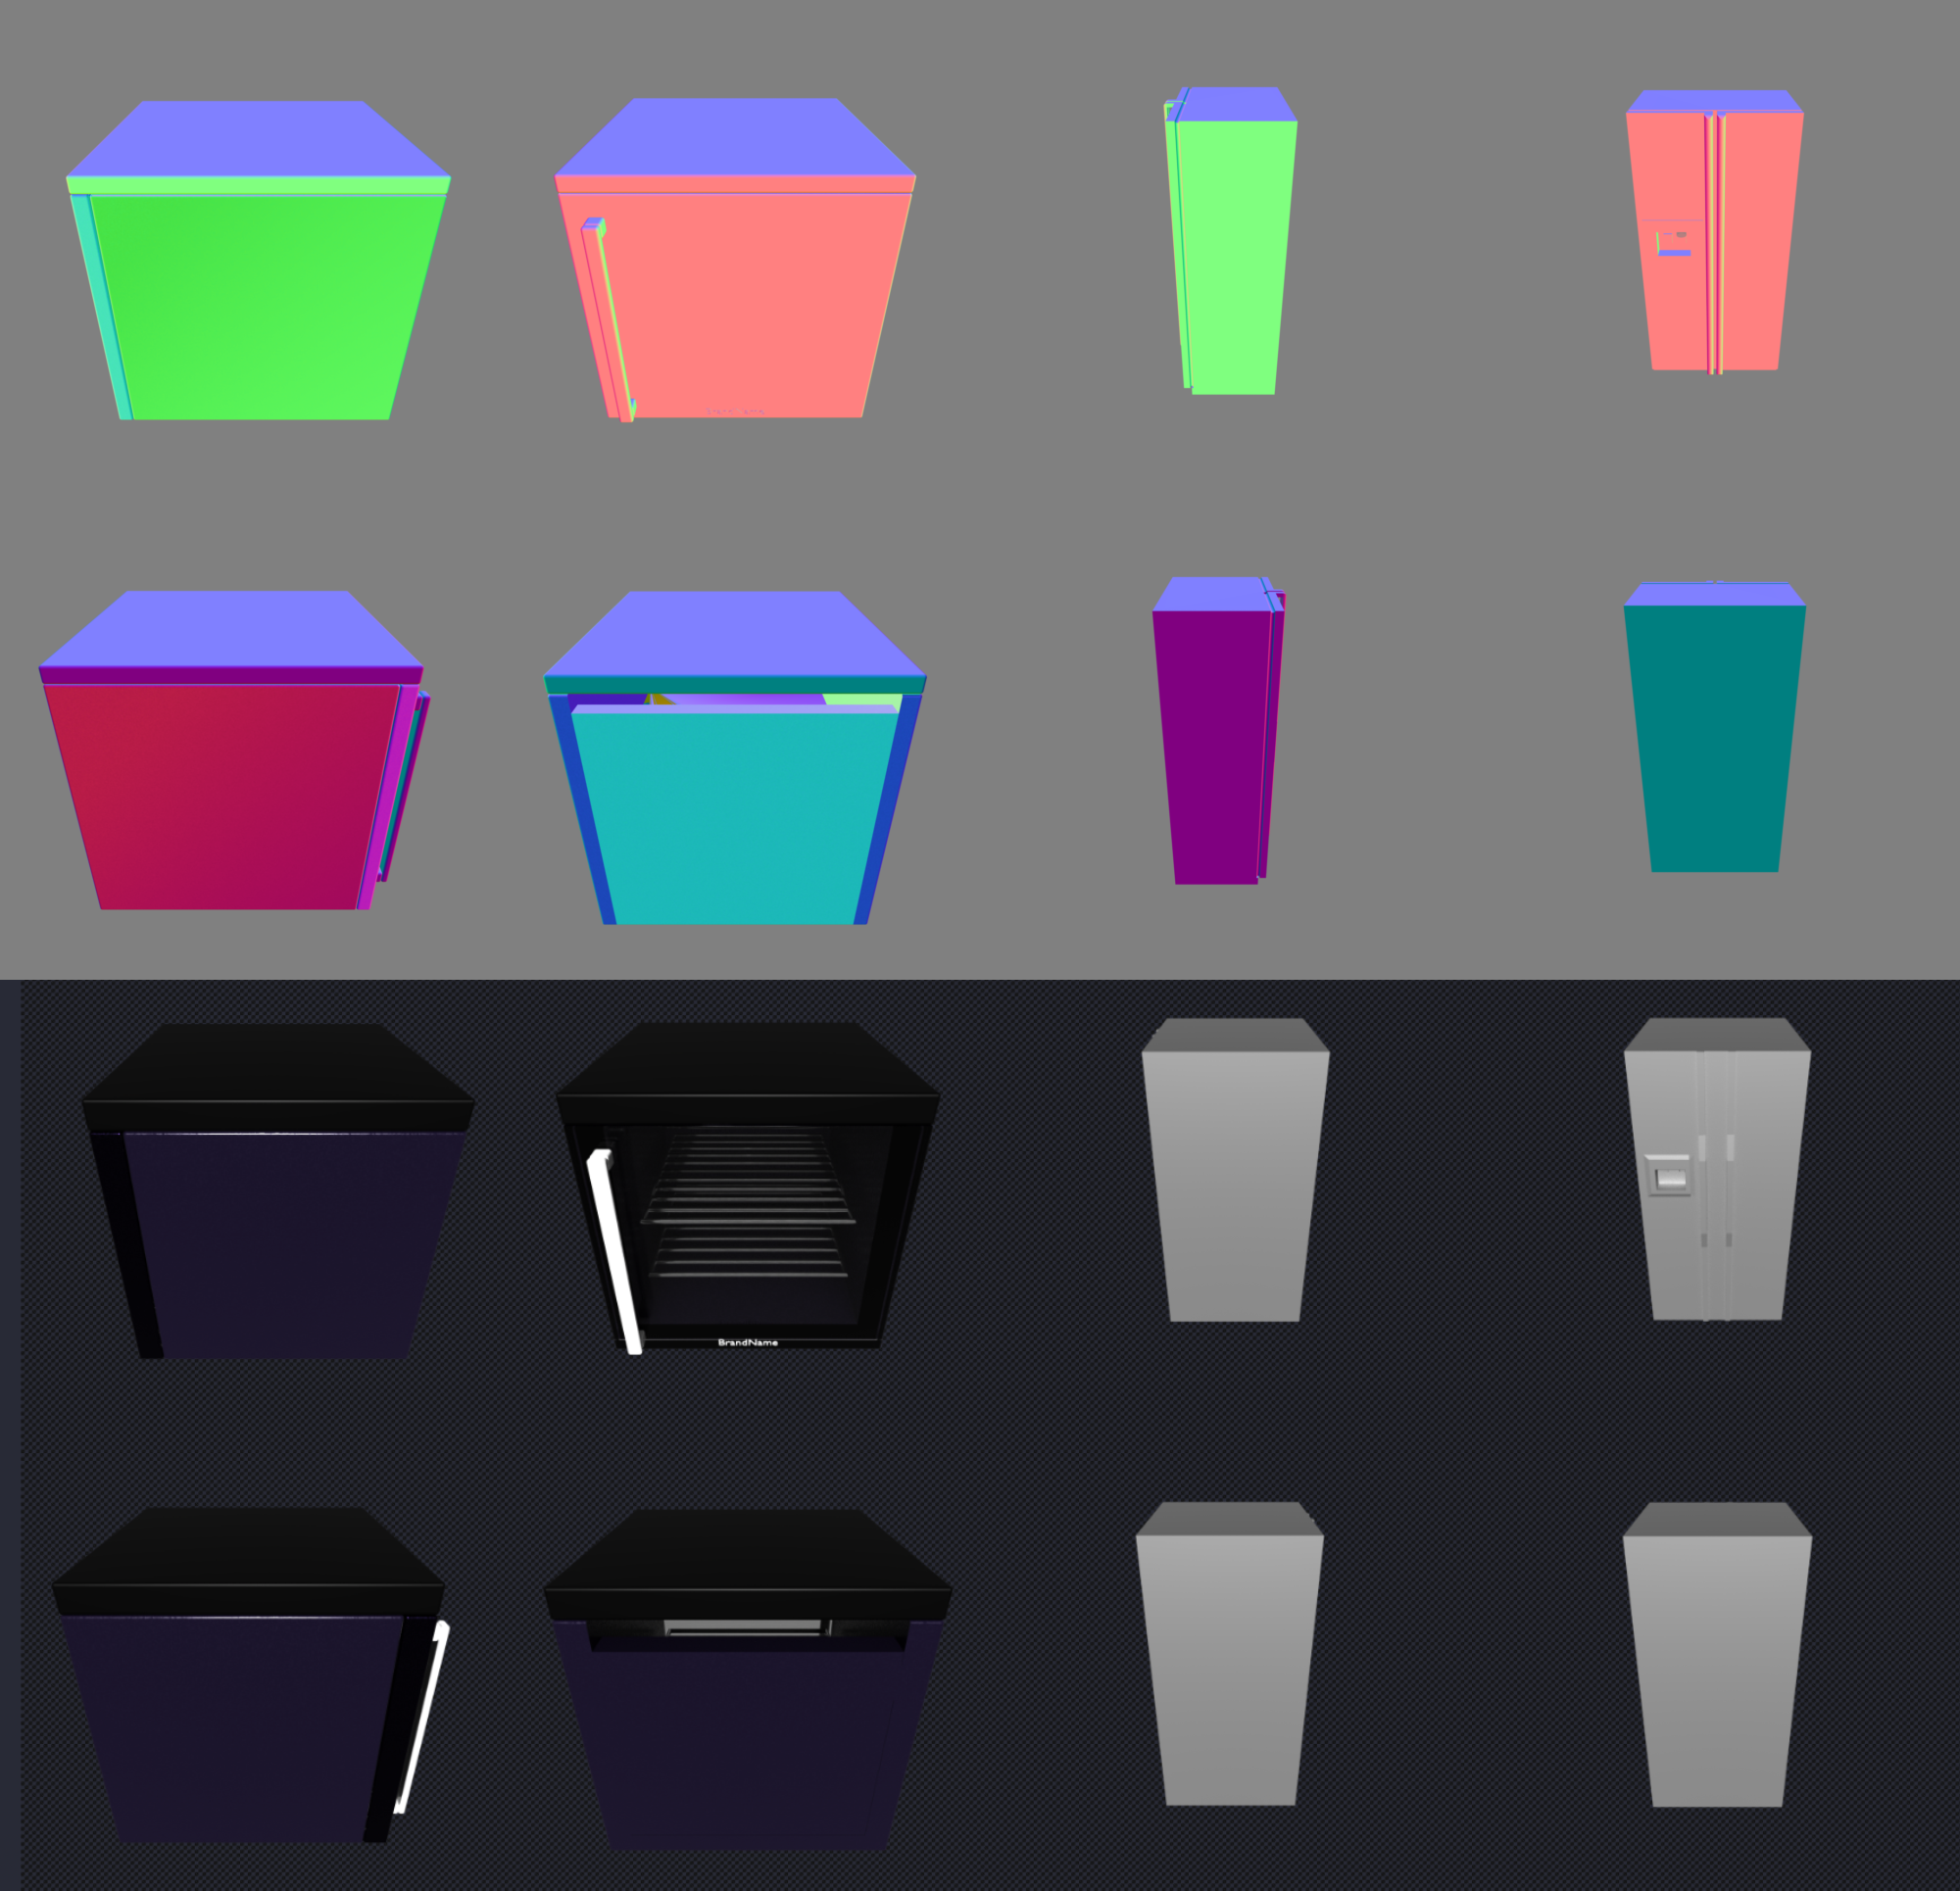}
    \caption{One sample pair for GPT4v evaluation.
    Upper row is the normal map and lower row is the RGB image.
    }
    \label{fig: gpt4v_samples}
\end{figure}
Prompt used to evaluate geometry of this sample and response from GPT4v is shown in Figure~\ref{fig: gpt4v_prompt_geo}.
\begin{figure*}[htbp]
    \centering
    \includegraphics[width=0.8\linewidth]{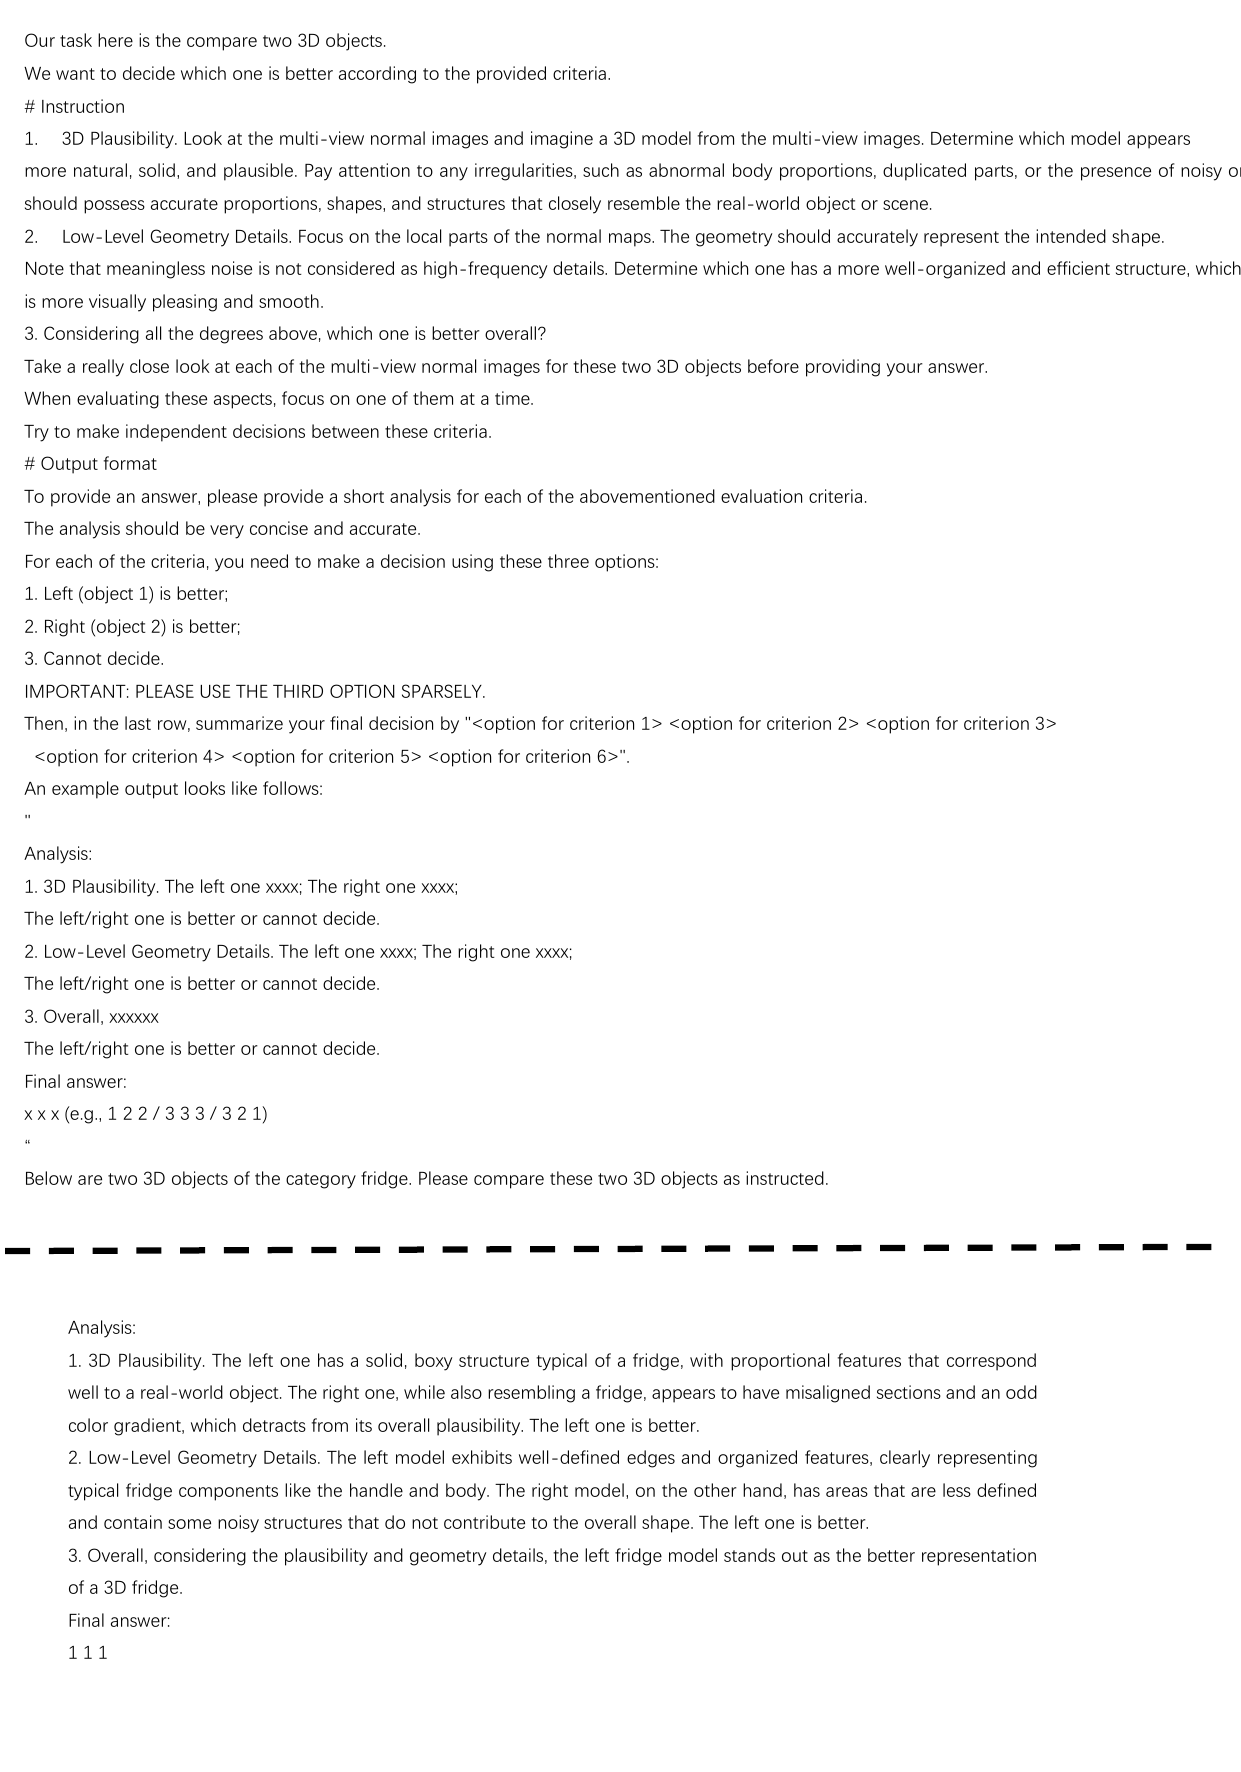}
    \caption{Prompt for GPT4v geometry evaluation and its response.}
    \label{fig: gpt4v_prompt_geo}
\end{figure*}
Prompt used to evaluate texture of this sample and response from GPT4v is shown in Figure~\ref{fig: gpt4v_prompt_tex}.
\begin{figure*}[htbp]
    \centering
    \includegraphics[width=0.8\linewidth]{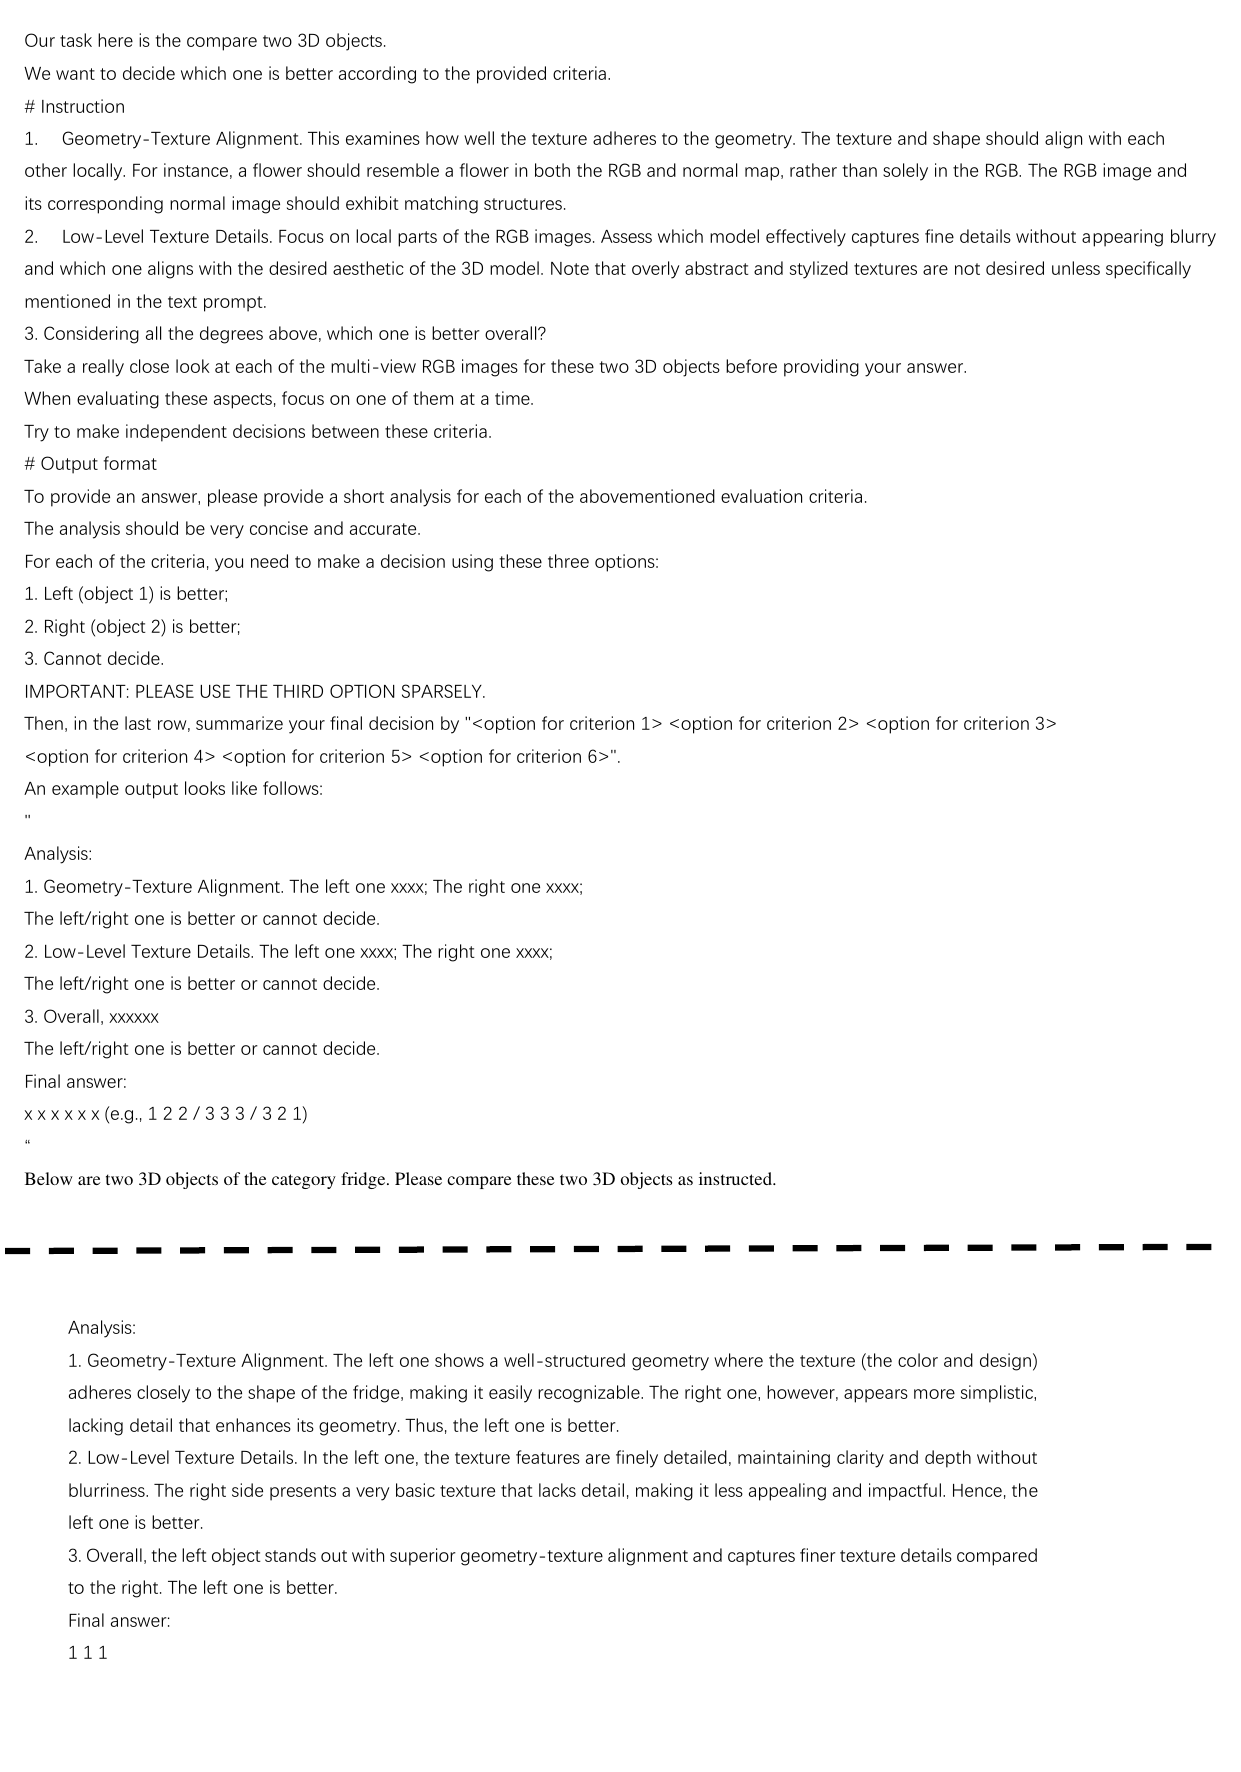}
    \caption{Prompt for GPT4v texture evaluation and its response.}
    \label{fig: gpt4v_prompt_tex}
\end{figure*}

\begin{figure*}[!h]
    \centering
    \includegraphics[width=0.9\textwidth]{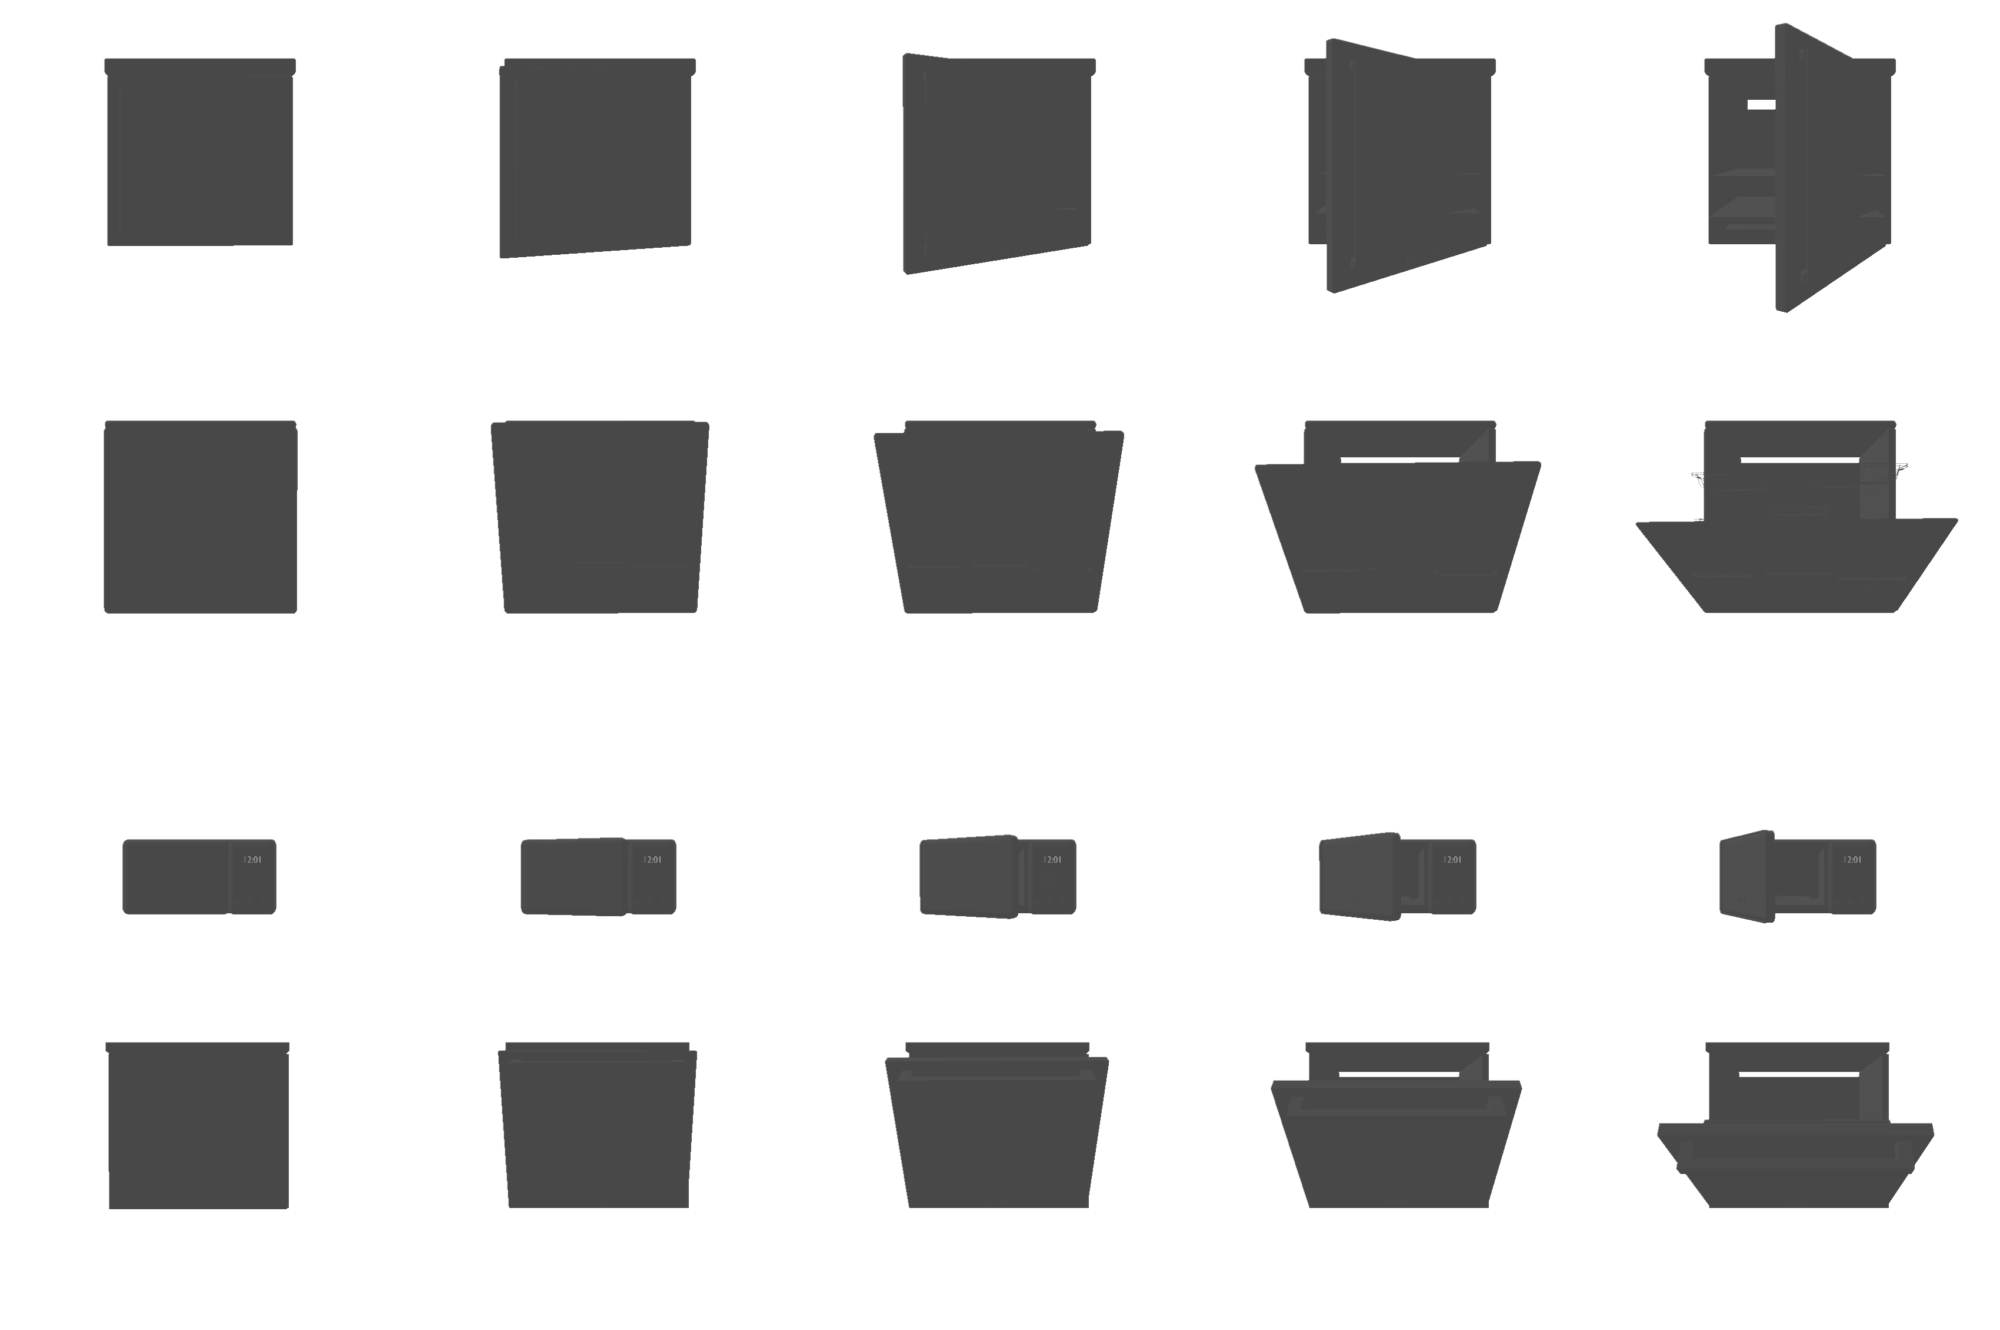}
    \caption{Motion sequences of samples generated by CAGE trained with our results.
    Each row shows the motion sequence of a sample.
    }
    \label{fig: cage_samples}
\end{figure*}

\section{Training Generative Models}
In this section we provide the details of training CAGE using our results.
We use the code implemented by the author with only the max node number adjusted to 256 to fit our results.
We display more motion sequences of samples generated by CAGE in Figure~\ref{fig: cage_samples}.
