# Supplementary material for: Infinite Mobility: Scalable High-Fidelity Synthesis of Articulated Objects via Procedural Generation
Source: arXiv:2503.13424 source file (2025-03-17)
Supplement: Supplementary file 2 [file suppl.pdf]

# Appendices

## A. All Categories We Support

In this section, we provide the list of all categories we support in Infinite Mobility till now. Based on frequency of interactions we observed and difficulty of implementation, we selected 22 categories of objects.

- Cabinet
- Pan
- Pot
- TV(Display)
- Dishwasher
- Microwave
- Fridge
- Oven
- Bar Chair
- Office Chair
- Window
- Lamp
- Tap
- Toilet
- Hardware
- Door
- Rack
- Cocktail Table
- Dining Table
- Plate Rack
- Bottle
- Vase

## B. Detail of Human Evaluation

In this section, we provide the details in the human evaluation. When completing the evaluation, the annotators were asked to answer the following question after watching each pair of videos . For each category, we construct 50 pairs of videos for evaluation. For PartNet-Mobility, if sample in one category is not available, we may use one sample for multiple times. For NAP, due to that it can't be conditioned on categories, we randomly select 50 samples from all categories.

**Please judge if the movement of joints in the video is physically plausible.**

**A. Left one is better.**

**B. Righr one is better.**

**C. Performances are tied and you can't tell which is better.**

Figure 1: Question used in human evaluation.

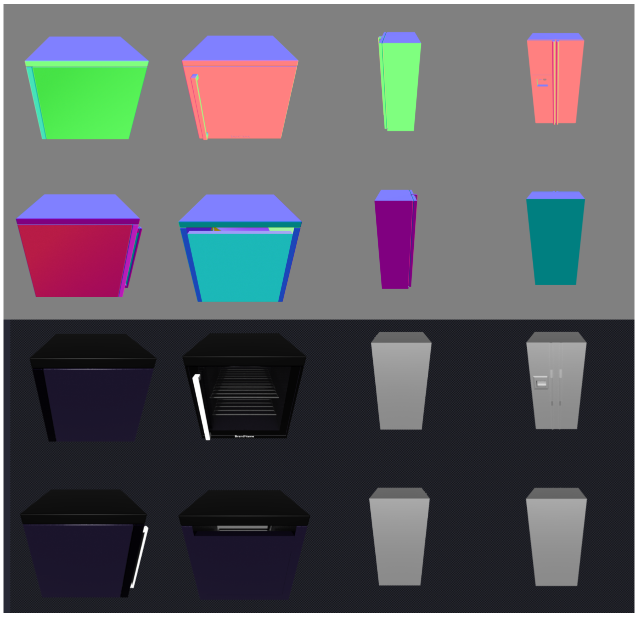

Figure 2: One sample pair for GPT4v evaluation. Upper row is the normal map and lower row is the RGB image.

## C. Detail of GPT4v Evaluation

In this section, we provide the details of the evaluation of mesh quality using GPT4v. We render normal maps and RGB images for each articulated object and construct paired samples for comparison. One sample pair is shown in Figure 2. Prompt used to evaluate geometry of this sample and response from GPT4v is shown in Figure 3. Prompt used to evaluate texture of this sample and response from GPT4v is shown in Figure 4.

## D. Training Generative Models

In this section we provide the details of training CAGE using our results. We use the code implemented by the author with only the max node number adjusted to 256 to fit our results. We display more motion sequences of samples generated by CAGE in Figure 5.

Our task here is the compare two 3D objects.
We want to decide which one is better according to the provided criteria.
# Instruction
1. 3D Plausibility. Look at the multi-view normal images and imagine a 3D model from the multi-view images. Determine which model appears more natural, solid, and plausible. Pay attention to any irregularities, such as abnormal body proportions, duplicated parts, or the presence of noisy o should possess accurate proportions, shapes, and structures that closely resemble the real-world object or scene.
2. Low-Level Geometry Details. Focus on the local parts of the normal maps. The geometry should accurately represent the intended shape. Note that meaningless noise is not considered as high-frequency details. Determine which one has a more well-organized and efficient structure, which is more visually pleasing and smooth.
3. Considering all the degrees above, which one is better overall?
Take a really close look at each of the multi-view normal images for these two 3D objects before providing your answer.
When evaluating these aspects, focus on one of them at a time.
Try to make independent decisions between these criteria.
# Output format
To provide an answer, please provide a short analysis for each of the abovementioned evaluation criteria.
The analysis should be very concise and accurate.
For each of the criteria, you need to make a decision using these three options:
1. Left (object 1) is better;
2. Right (object 2) is better;
3. Cannot decide.
IMPORTANT: PLEASE USE THE THIRD OPTION SPARSELY.
Then, in the last row, summarize your final decision by "<option for criterion 1> <option for criterion 2> <option for criterion 3> <option for criterion 4> <option for criterion 5> <option for criterion 6>".
An example output looks like follows:
"
Analysis:
1. 3D Plausibility. The left one xxxx; The right one xxxx;
The left/right one is better or cannot decide.
2. Low-Level Geometry Details. The left one xxxx; The right one xxxx;
The left/right one is better or cannot decide.
3. Overall, xxxxxx
The left/right one is better or cannot decide.
Final answer:
x x x (e.g., 1 2 2 / 3 3 3 / 3 2 1)
"
Below are two 3D objects of the category fridge. Please compare these two 3D objects as instructed.

---

Analysis:
1. 3D Plausibility. The left one has a solid, boxy structure typical of a fridge, with proportional features that correspond well to a real-world object. The right one, while also resembling a fridge, appears to have misaligned sections and an odd color gradient, which detracts from its overall plausibility. The left one is better.
2. Low-Level Geometry Details. The left model exhibits well-defined edges and organized features, clearly representing typical fridge components like the handle and body. The right model, on the other hand, has areas that are less defined and contain some noisy structures that do not contribute to the overall shape. The left one is better.
3. Overall, considering the plausibility and geometry details, the left fridge model stands out as the better representation of a 3D fridge.
Final answer:
1 1 1

Figure 3: Prompt for GPT4v geometry evaluation and its response.

Our task here is the compare two 3D objects.
We want to decide which one is better according to the provided criteria.
# Instruction
1. Geometry-Texture Alignment. This examines how well the texture adheres to the geometry. The texture and shape should align with each other locally. For instance, a flower should resemble a flower in both the RGB and normal map, rather than solely in the RGB. The RGB image and its corresponding normal image should exhibit matching structures.
2. Low-Level Texture Details. Focus on local parts of the RGB images. Assess which model effectively captures fine details without appearing blurry and which one aligns with the desired aesthetic of the 3D model. Note that overly abstract and stylized textures are not desired unless specifically mentioned in the text prompt.
3. Considering all the degrees above, which one is better overall?
Take a really close look at each of the multi-view RGB images for these two 3D objects before providing your answer.
When evaluating these aspects, focus on one of them at a time.
Try to make independent decisions between these criteria.
# Output format
To provide an answer, please provide a short analysis for each of the abovementioned evaluation criteria.
The analysis should be very concise and accurate.
For each of the criteria, you need to make a decision using these three options:
1. Left (object 1) is better;
2. Right (object 2) is better;
3. Cannot decide.
IMPORTANT: PLEASE USE THE THIRD OPTION SPARSELY.
Then, in the last row, summarize your final decision by "<option for criterion 1> <option for criterion 2> <option for criterion 3> <option for criterion 4> <option for criterion 5> <option for criterion 6>".
An example output looks like follows:
"
Analysis:
1. Geometry-Texture Alignment. The left one xxxx; The right one xxxx;
The left/right one is better or cannot decide.
2. Low-Level Texture Details. The left one xxxx; The right one xxxx;
The left/right one is better or cannot decide.
3. Overall, xxxxxx
The left/right one is better or cannot decide.
Final answer:
x x x x x x (e.g., 1 2 2 / 3 3 3 / 3 2 1)
"
Below are two 3D objects of the category fridge. Please compare these two 3D objects as instructed.

Analysis:
1. Geometry-Texture Alignment. The left one shows a well-structured geometry where the texture (the color and design) adheres closely to the shape of the fridge, making it easily recognizable. The right one, however, appears more simplistic, lacking detail that enhances its geometry. Thus, the left one is better.
2. Low-Level Texture Details. In the left one, the texture features are finely detailed, maintaining clarity and depth without blurriness. The right side presents a very basic texture that lacks detail, making it less appealing and impactful. Hence, the left one is better.
3. Overall, the left object stands out with superior geometry-texture alignment and captures finer texture details compared to the right. The left one is better.
Final answer:
1 1 1

Figure 4: Prompt for GPT4v texture evaluation and its response.

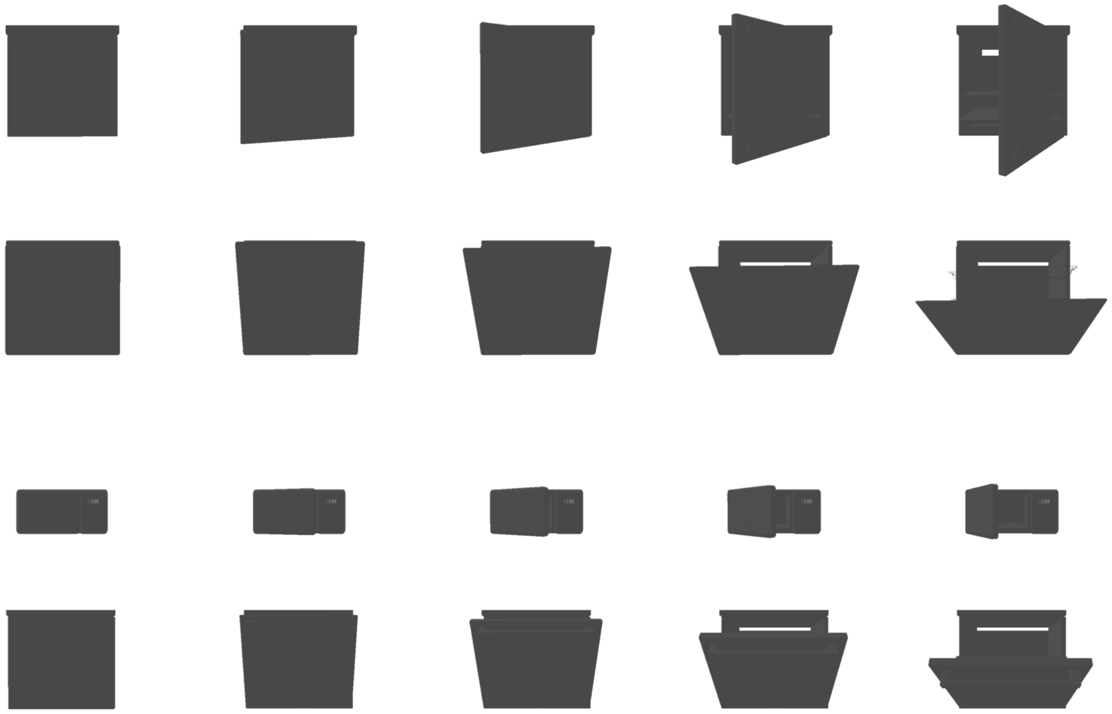

Figure 5: Motion sequences of samples generated by CAGE trained with our results. Each row shows the motion sequence of a sample.
